# Supplementary material for: AEDFL: Efficient Asynchronous Decentralized Federated Learning with Heterogeneous Devices
Source: arXiv:2312.10935 source file (2023-12-18)
Supplement: Supplementary file 1 [file AppendixFile.tex]

\documentclass{article} % For LaTeX2e
\usepackage{ltexpprt}

\usepackage{times}
\usepackage{soul}
\usepackage[hidelinks]{hyperref}
\usepackage[utf8]{inputenc}
\usepackage[small]{caption}
\usepackage{textpos}
\usepackage{textcomp}
\usepackage{xcolor}
\usepackage{bigstrut}

\usepackage{algorithm}
\usepackage{algorithmic}
\usepackage{hyperref}
\usepackage{url}
\usepackage{graphicx}
\usepackage{subfigure} 
\usepackage{amsfonts}
\usepackage{amssymb}
\usepackage{amsthm}
\usepackage{mathrsfs}
\usepackage{booktabs}
\usepackage{multirow}
\usepackage{multicol}
\usepackage{mathrsfs}
\usepackage{amsmath,amssymb,amsfonts}
\usepackage[switch]{lineno}

\usepackage{chngcntr}

% The \author macro works with any number of authors. There are two commands
% used to separate the names and addresses of multiple authors: \And and \AND.
%
% Using \And between authors leaves it to \LaTeX{} to determine where to break
% the lines. Using \AND forces a linebreak at that point. So, if \LaTeX{}
% puts 3 of 4 authors names on the first line, and the last on the second
% line, try using \AND instead of \And before the third author name.

%\iclrfinalcopy % Uncomment for camera-ready version, but NOT for submission.
\begin{document}

\input{Appendix.tex}

\bibliographystyle{named}
\bibliography{ref}

\end{document}
